# Supplementary material for: StyleSpeaker: Audio-Enhanced Fine-Grained Style Modeling for Speech-Driven 3D Facial Animation
Source: arXiv:2503.09852 source file (2025-03-12)
Supplement: Supplementary file 1 [file X_suppl.tex]

\clearpage
\setcounter{page}{1}
\maketitlesupplementary
Our supplementary material includes a video and an appendix. We introduce the appendix below.
\section*{Appendix}
\appendix
This appendix contains three sections: Section~\ref{A} shows the details of StyleSpeaker in hyper-parameters, model architecture, comparisons with baselines, and user study; Section~\ref{B} shows the details of 3D-MEAD; 
% Section~\ref{C} shows the  example analyses for audio enhancement; 
Section~\ref{C} presents short descriptions for our supplementary video. 
% We include our model code in the supplementary material and will release the full code and weights publicly at a later time.
\section{Details of StyleSpeaker}
\label{A}
\subsection{Hyper-parameters}
The feature dimensions $d_a$, $d_s$ and $d_m$ are all set to 256. The value of $k$ is set to 5, which controls the calculation range of local contrastive loss. The number of style primitives $e$ is set to 8. 

\subsection{Details of Model Architecture}
\paragraph{Speaker Style Extractor.}
We introduce the detailed structure of the speaker style extractor, as shown in Figure \ref{motion}.
Specifically, we first project the face motion sequence $\mathbf{M}_{1:T}$ into a $d_s$-dimensional space via a mesh encoder and extract features from the projected sequence using a temporal convolutional network (TCN). We then calculate the mean, standard deviation, and first-order difference standard deviation of the features along the temporal dimension, and concatenate them into a composite vector. We feed the composite vector into a fully connected (FC) layer to obtain $S_r$. We set the number of temporal convolution blocks $N_r = 4$ in our experiments.
\begin{figure}[b]
\centering
\includegraphics[width=1.0\linewidth]{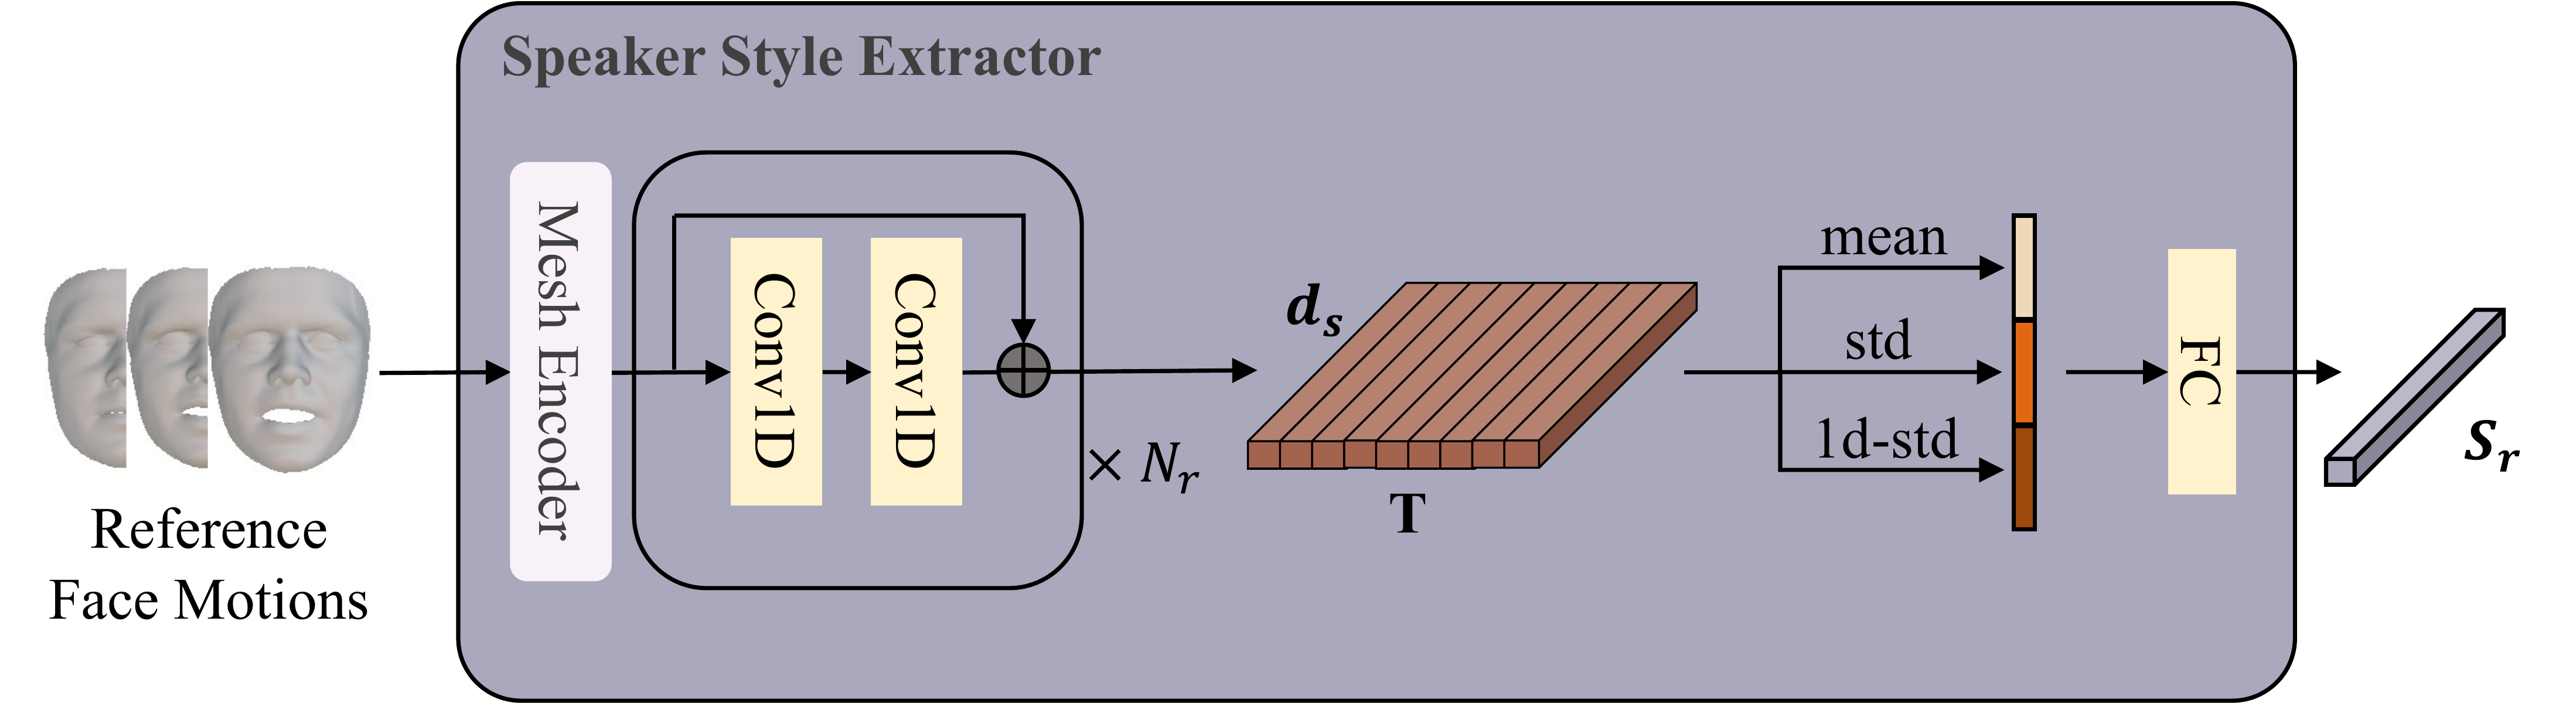}
\caption{Visualization of the speaker style extractor structure.}
\label{motion}
\end{figure}

\paragraph{Audio Condition Extractor.} \vspace{-\baselineskip}
The audio condition extractor has a similar structure to the speaker style extractor, as shown in Figure \ref{audio}. We use the maximum value instead of the average value because we are concerned with the deviations provided by the audio features.  We set $N_a = 4$ in our experiments.
\begin{figure}[t]
\centering
\includegraphics[width=1.0\linewidth]{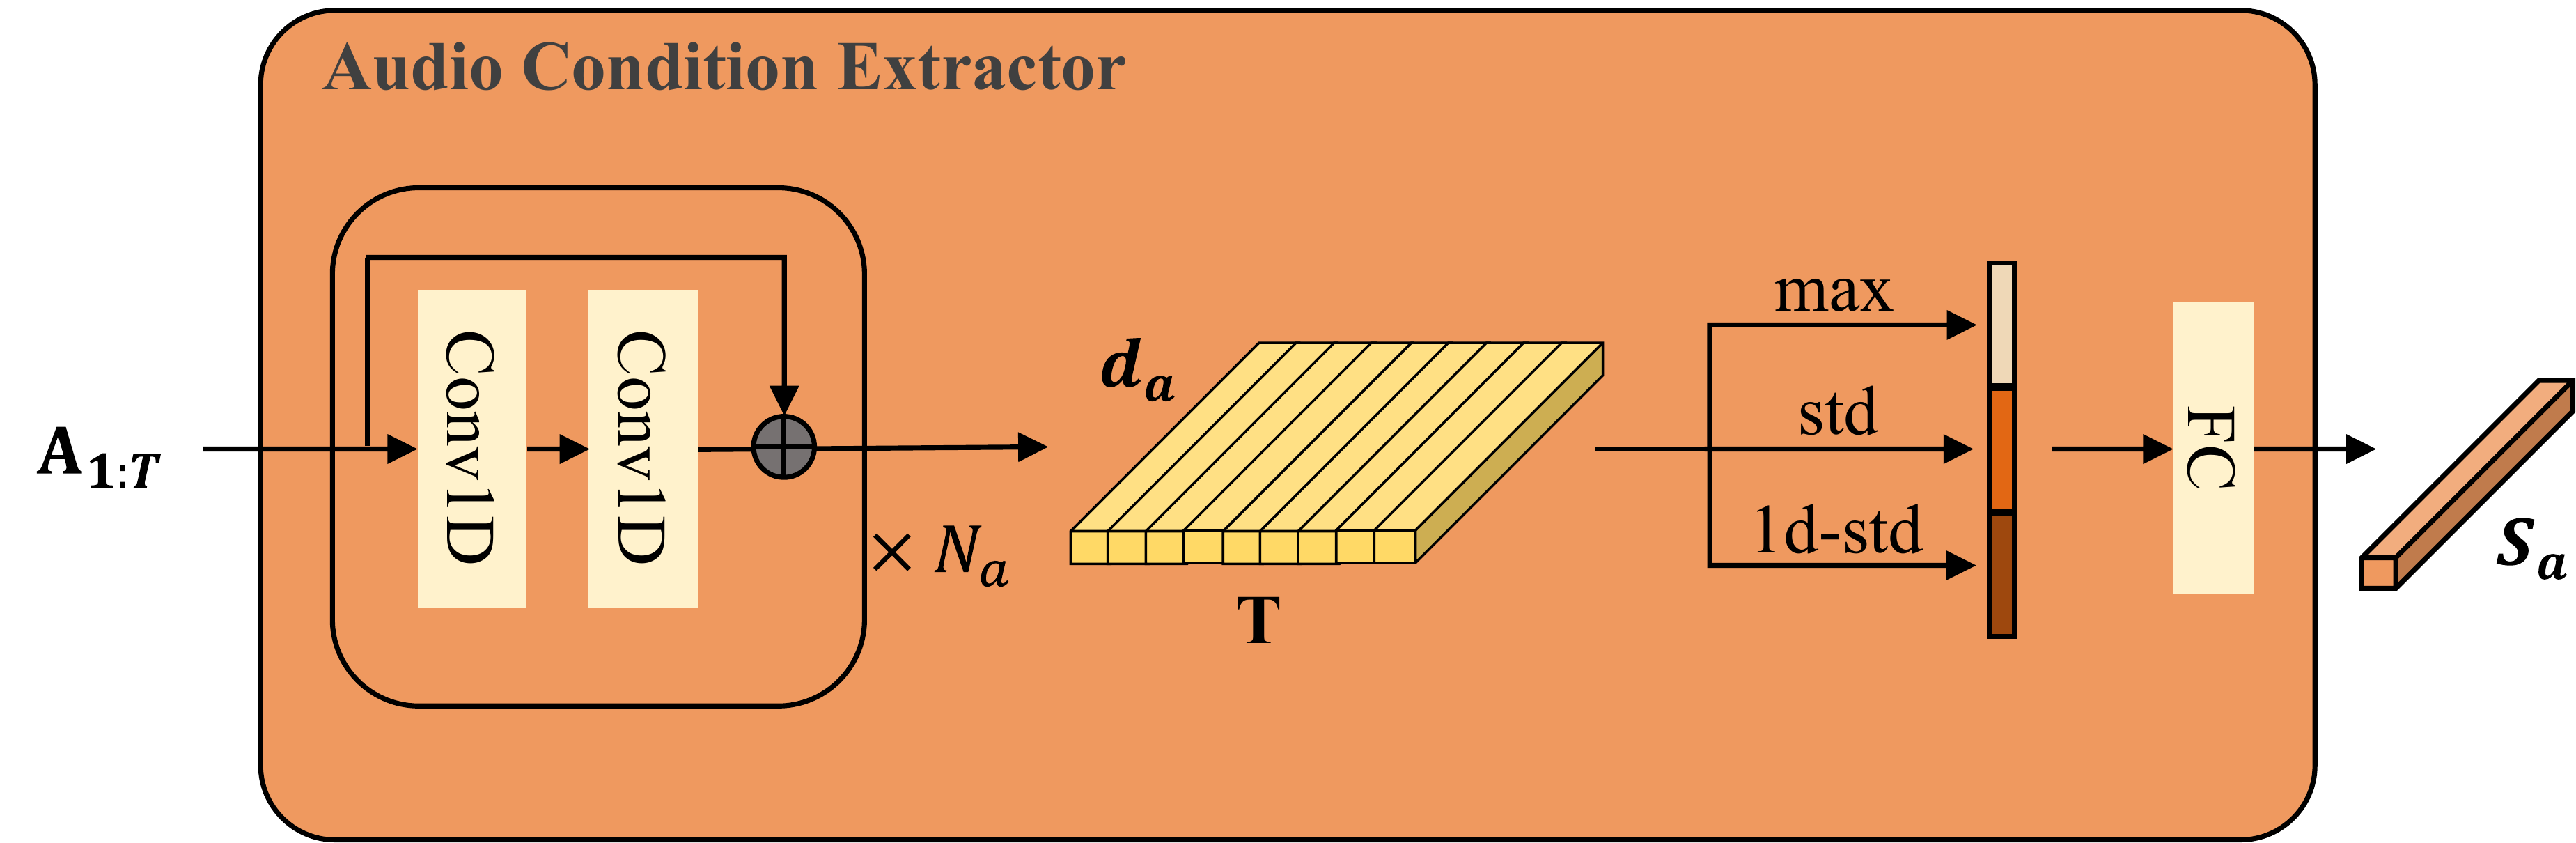} % Reduce the figure size so that it is slightly narrower than the column.
\caption{Visualization of the audio condition extractor structure.}
\label{audio}
\end{figure}
\subsection{Details of Comparison}
We compare our method with FaceFormer~\cite{fan2022faceformer}, CodeTalker~\cite{xing2023codetalker}, FaceDiffuser~\cite{stan2023facediffuser}, and CorrTalk~\cite{chu2024corrtalk} on BIWI-Test-A, BIWI-Test-B, and VOCASET-Test. For these competing methods, we use the official inference code and model weights to obtain the best results in the original paper. We compare our method with Imitator~\cite{thambiraja2023imitator} and Mimic~\cite{fu2024mimic} on MEAD-Test-A and MEAD-Test-B.
We use the official training code to train Imitator and Mimic on MEAD-Train. Imitator uses the model weights of the 59-th epoch for testing under the early stopping mechanism. For Mimic, we observe that the training process has converged, and we conduct the test using the model weights of the 80-th epoch, with a training duration that is 5.6 times longer than that of our method.

For the comparison on MEAD-Test-B, we select the same one 3D facial sequence and the corresponding speech from the target speaker, as a reference for all methods. Afterward, we test on the remaining data. Our method and Mimic do not require speech and fine-tuning. Imitator requires speech and needs to be fine-tuned for 600 epochs.
\subsection{Details of User Study}
We design our user study interface, as shown in Figure~\ref{user_study1} and ~\ref{user_study2}. For BIWI-Test-B and VOCASET-Test, each participant is asked to answer two questions: ``Which video has better lip synchronization?'' and ``Which video has better realism?''  For MEAD-Test-B, after answering the above two questions, each participant is also asked to answer the third question: ``Which video has a more consistent speaking style with the leftmost GT video?'' based on the comparison with the GT video. Each participant answers 15, 15 and 10 questions for BIWI-Test-B, VOCASET-Test and MEAD-Test-B, respectively.

\begin{figure}[h]
\centering
\includegraphics[width=1.0\linewidth]{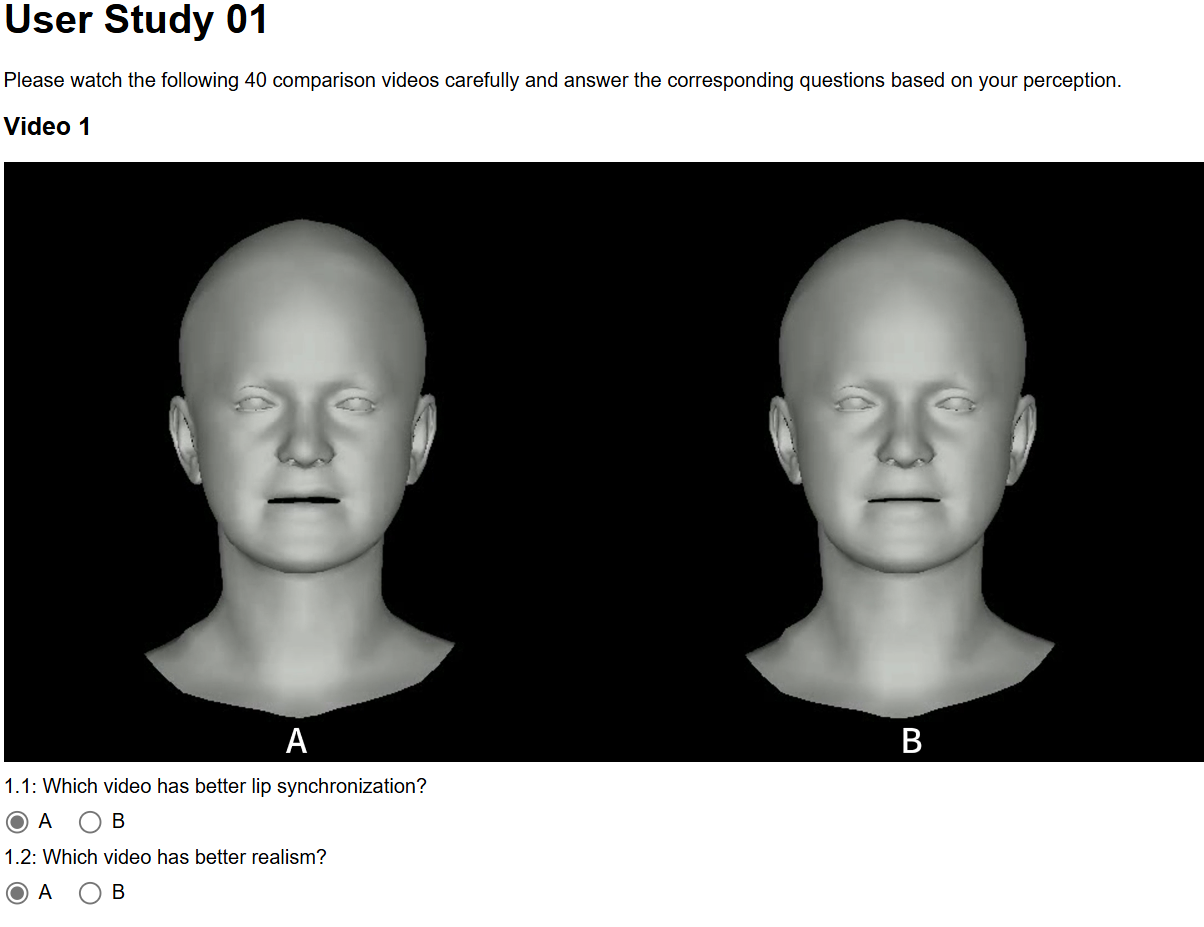} % Reduce the figure size so that it is slightly narrower than the column.
\caption{Interaction interface of the user study (type 1).}
\label{user_study1}
\end{figure}

\begin{figure}[h]
\centering
\includegraphics[width=1.0\linewidth]{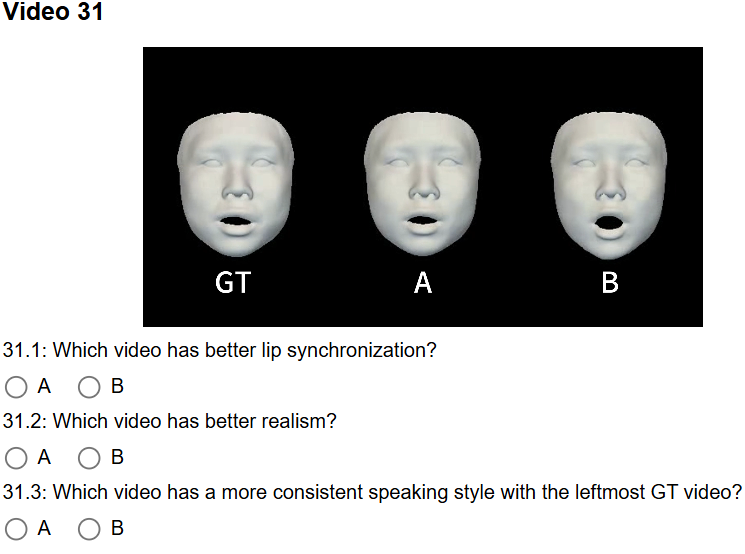} % Reduce the figure size so that it is slightly narrower than the column.
\caption{Interaction interface of the user study (type 2).}
\label{user_study2}
\end{figure}

\section{Details of 3D-MEAD}
\label{B}
3D-MEAD is synthesized by HRN~\cite{lei2023hierarchical} based on MEAD dataset~\cite{wang2020mead}.
MEAD is a talking-face video corpus featuring 60 actors talking with eight different emotions at three different levels. In this paper, we use the neutral emotion and frontal view. HRN is a 3D facial reconstruction method based on 3D morphable model (3DMM)~\cite{blanz2023morphable, romdhani2005estimating}, capable of synthesizing three levels of 3D facial geometry: low, middle, and high, corresponding to different levels of detail. 
We synthesize pseudo ground truth for middle-level 3D facial geometry sequences.

\section{Supplementary Video}
\label{C}
Our supplementary video consists of three parts.
In part 1, we present comparative examples with competing methods for seen speakers on VOCASET-Test, BIWI-Test-A, and MEAD-Test-A. In part 2, we provide comparative examples with competing methods for unseen speakers on MEAD-Test-B, based on the same reference videos. In part 3, we show comparative examples from the ablation experiments targeting the removal of the style primitives.

%说的再详细点！！！！！！！！！！
